# Supplementary material for: Magnetocaloric effect and its electric-field regulation in CrI$_3$/metal heterostructure
Source: arXiv:2304.12582 source file (2023-04-25)
Supplement: Supplementary file 1 [file SI.pdf]

# Supplementary information

# Magnetocaloric effect and its electric-field regulation in $CrI_3$/metal heterostructure

Weiwei He,[†,¶] Ziming Tang,[†,¶] Qihua Gong,[*,†,‡] Min Yi,[*,†] and Wanlin Guo[†]

†*State Key Laboratory of Mechanics and Control for Aerospace Structures & Key Lab for Intelligent Nano Materials and Devices of Ministry of Education & Institute for Frontier Science, Nanjing University of Aeronautics and Astronautics (NUAA), Nanjing 210016, China*

‡*MIIT Key Laboratory of Aerospace Information Materials and Physics & College of Physics, Nanjing University of Aeronautics and Astronautics (NUAA), Nanjing 211106, China*

¶*Authors contributed equally.*

E-mail: gongqihua@nuaa.edu.cn; yimin@nuaa.edu.cn

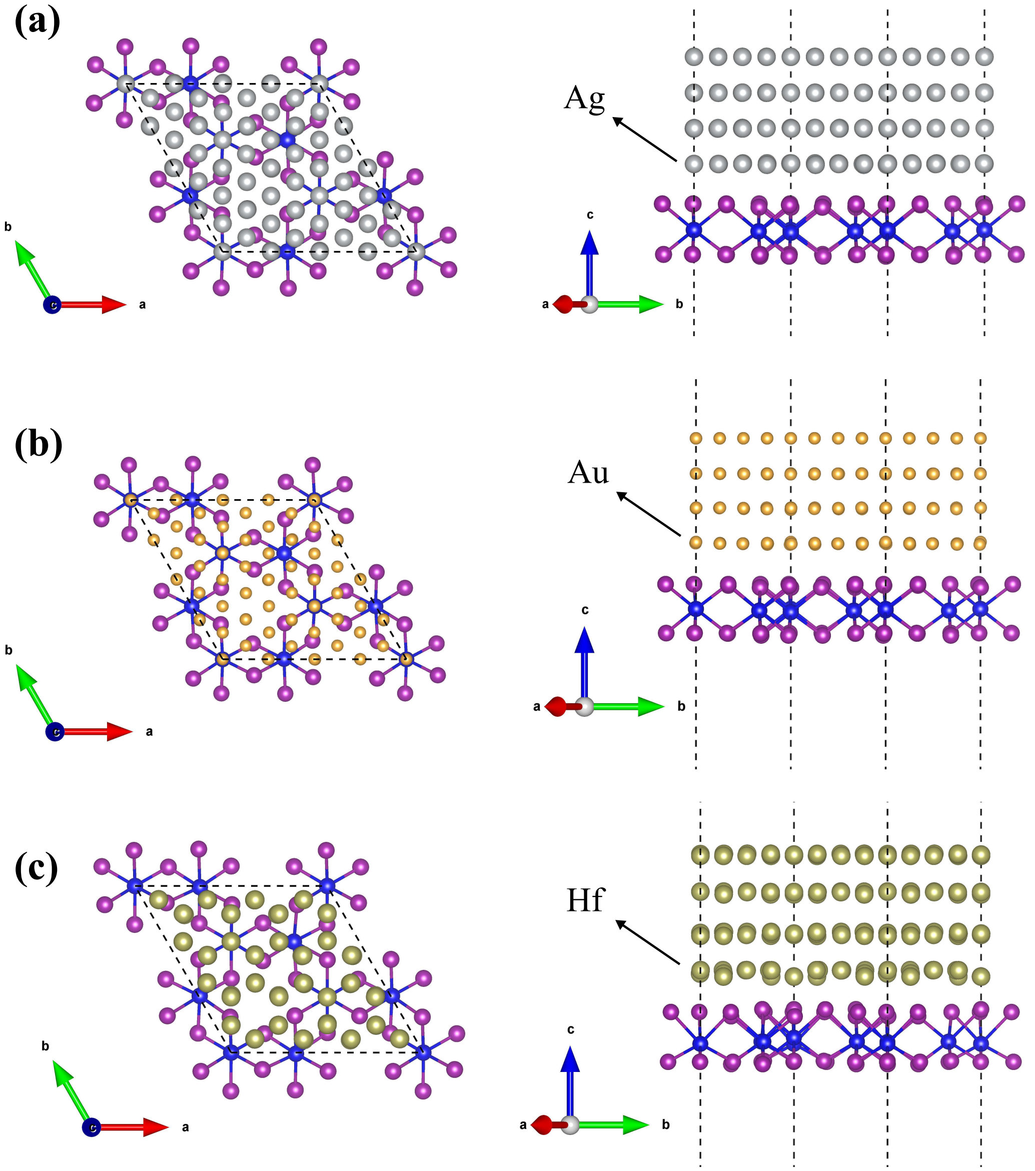


Fig. S1. Top and side views of $CrI_3$/metal vdW heterostructures: (a) $CrI_3$/Ag(111) configuration, (b) $CrI_3$/Au(111) configuration, and (c) $CrI_3$/Hf(001) configuration. The heterostructure of (a) $CrI_3$/Ag(111) and (b) $CrI_3$/Au(111) is built by placing a $2 \times 2$ supercell of Ag(111) and Au(111) on $\sqrt{3} \times \sqrt{3}$ unit cells of monolayer $CrI_3$. The heterostructure of (c) $CrI_3$/Hf(001) is built by placing a $4 \times 4$ supercell of Hf(001) on $\sqrt{3} \times \sqrt{3}$ unit cells of monolayer $CrI_3$. Silver, gold, greyish-green, purple, and purplish-blue balls represent Ag, Au, Hf, I, and Cr atoms, respectively.

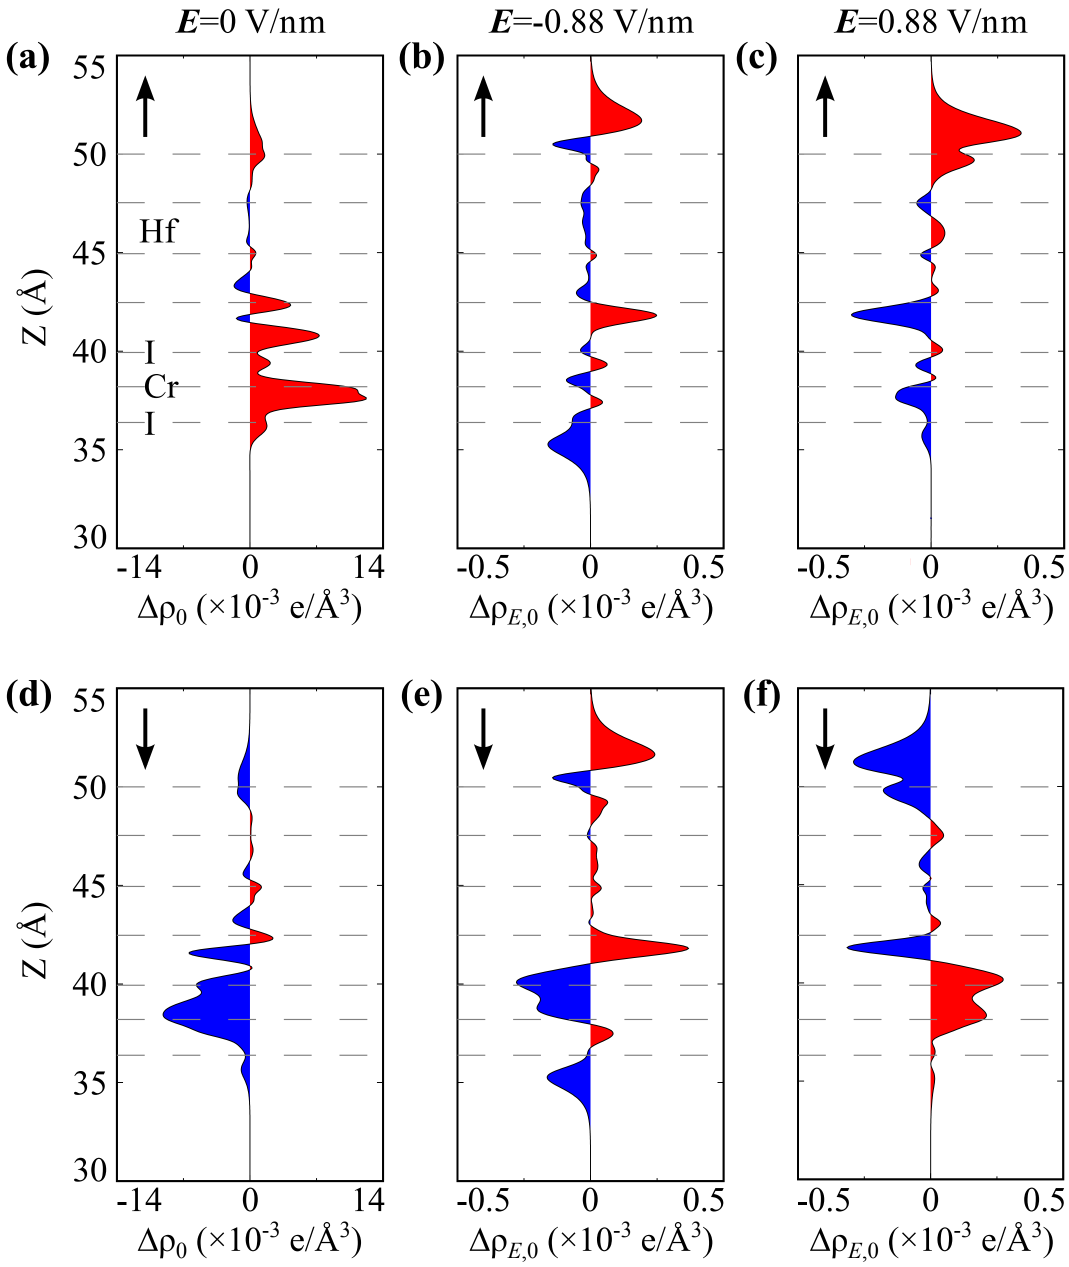


Fig. S2. Spin-dependent plane integrated charge density difference along $c/z$ direction. (a), (d) Plane averaged charge density difference $\Delta\rho_0$ of $CrI_3$/Hf without $E$ in spin-up (spin-down) direction. Using $\Delta\rho_0$ as a reference, the change $\Delta\rho_{E,0}$ represents charge density difference of $CrI_3$/Hf under different $E$. (b), (e) Spin-up (spin-down) charge with $E = -0.88\,\mathrm{V/nm}$. (c), (f) Spin-up (spin-down) charge with $E = 0.88\,\mathrm{V/nm}$. After forming the $CrI_3$/Hf interface, there is an accumulation of electrons in $CrI_3$ side in the spin-up channel while in the spin-down channel there exists a substantial depletion of electrons in (a) and (d). Such a charge redistribution leads to the stronger spin polarization, which unveils the reason that Hf substrate greatly improves the magenetic moment of Cr.[1] As depicted in (b) and (e), when the $CrI_3$/Hf is subjected to $E = -0.88\,\mathrm{V/nm}$, although the charge in both spin channels exhibit depletion at $CrI_3$, the more losses of spin-down charge render a net increase of magnetic moment of Cr.

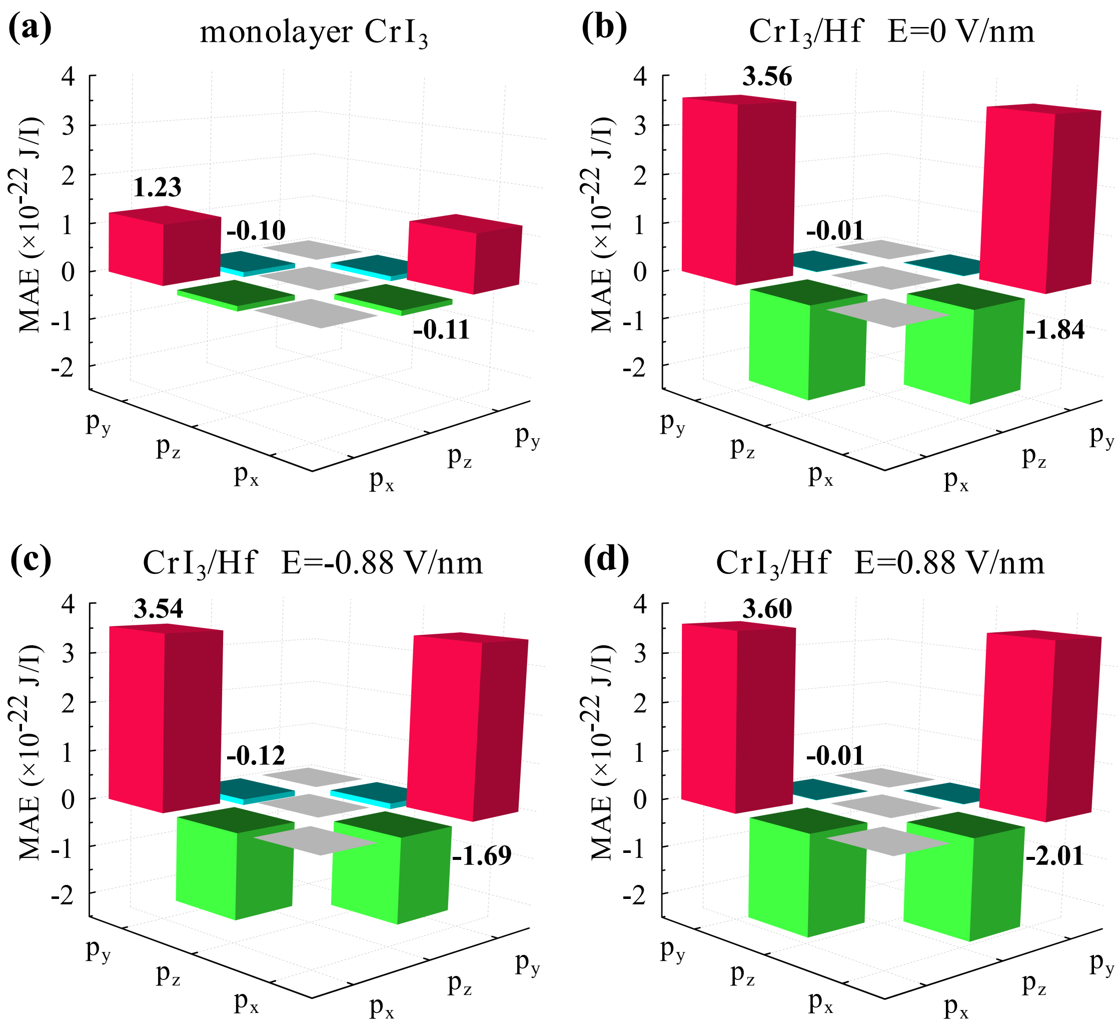


Fig. S3. The $p$-orbital resolved MAE of I atom in $CrI_3$: (a) monolayer $CrI_3$, (b) $CrI_3$ in $CrI_3$/Hf heterostructure without $E$, (c) $CrI_3$ in $CrI_3$/Hf heterostructure with $E = -0.88\,\mathrm{V/nm}$, and (d) $CrI_3$ in $CrI_3$/Hf heterostructure with $E = 0.88\,\mathrm{V/nm}$. Compared to monolayer $CrI_3$, the large rise in the positive contribution of matrix element differences ($p_x$, $p_y$) to perpendicular magnetic anisotropy in the $CrI_3$/Hf heterostructure compensates for the negative contribution from element differences ($p_x$, $p_z$), resulting in an improvement in MAE. As the strength of $E$ increases, there is a little increase in ($p_x$, $p_y$), but the negative contribution of ($p_x$, $p_z$) decreases more significantly, resulting in a decrease in MAE.

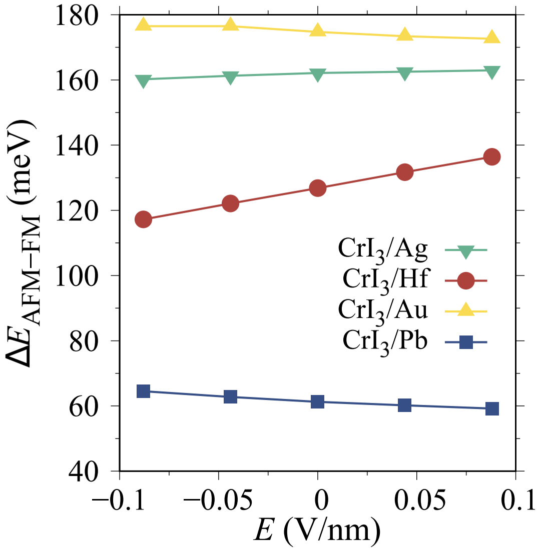


Fig. S4. Energy difference between FM and AFM configurations ($\Delta E_{\text{FM-AFM}}$) of $CrI_3$ as a function of $E$ in $CrI_3$/metal vdW heterostructures.

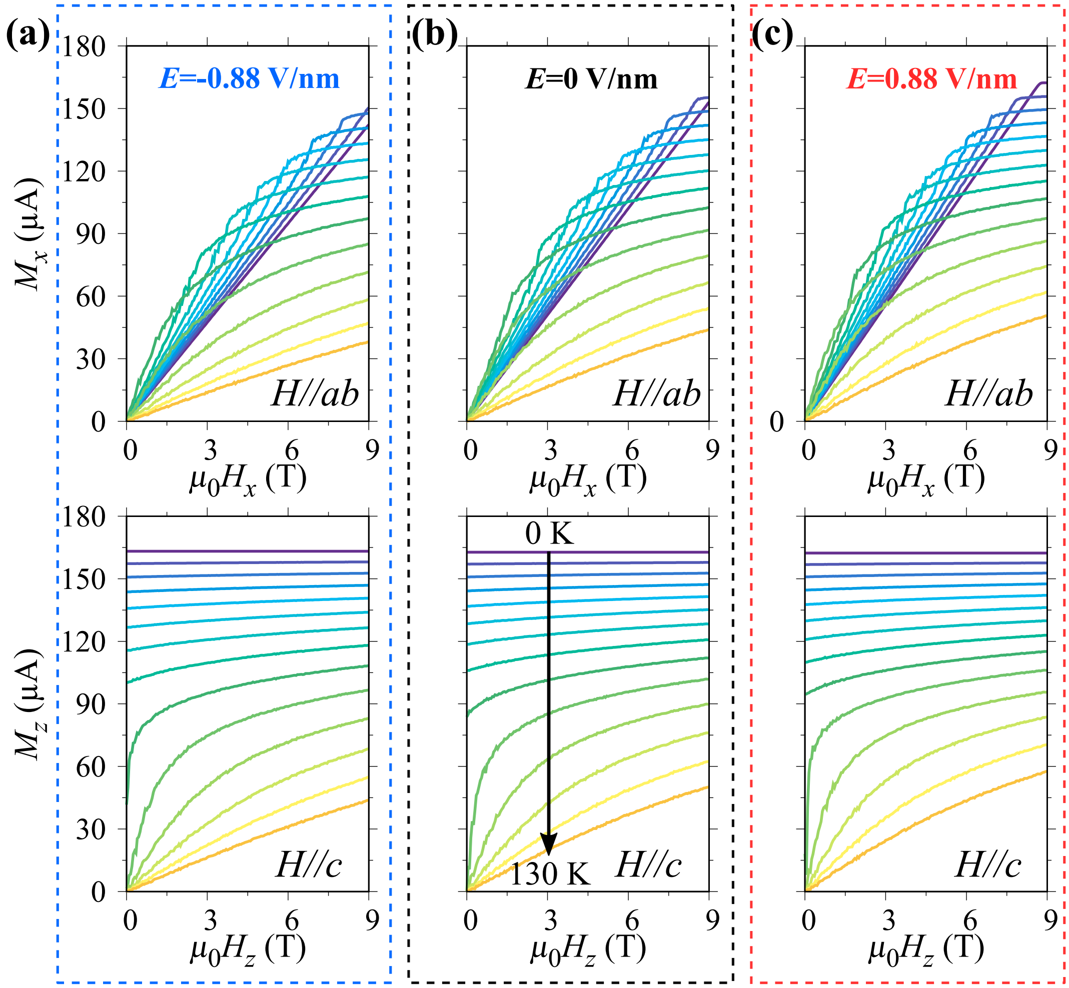


Fig. S5. Isothermal demagnetization curves of $CrI_3$ in $CrI_3$/Hf heterostructure under a field up to 9 T: (a) $E = -0.88$ V/nm, (b) $E = 0$ V/nm, and (c) $E = 0.88$ V/nm. The magnetic field direction is applied along the in-plane (top-row subfigures) and out-of-plane (bottom-row subfigures). The curves are displayed every 10 K.

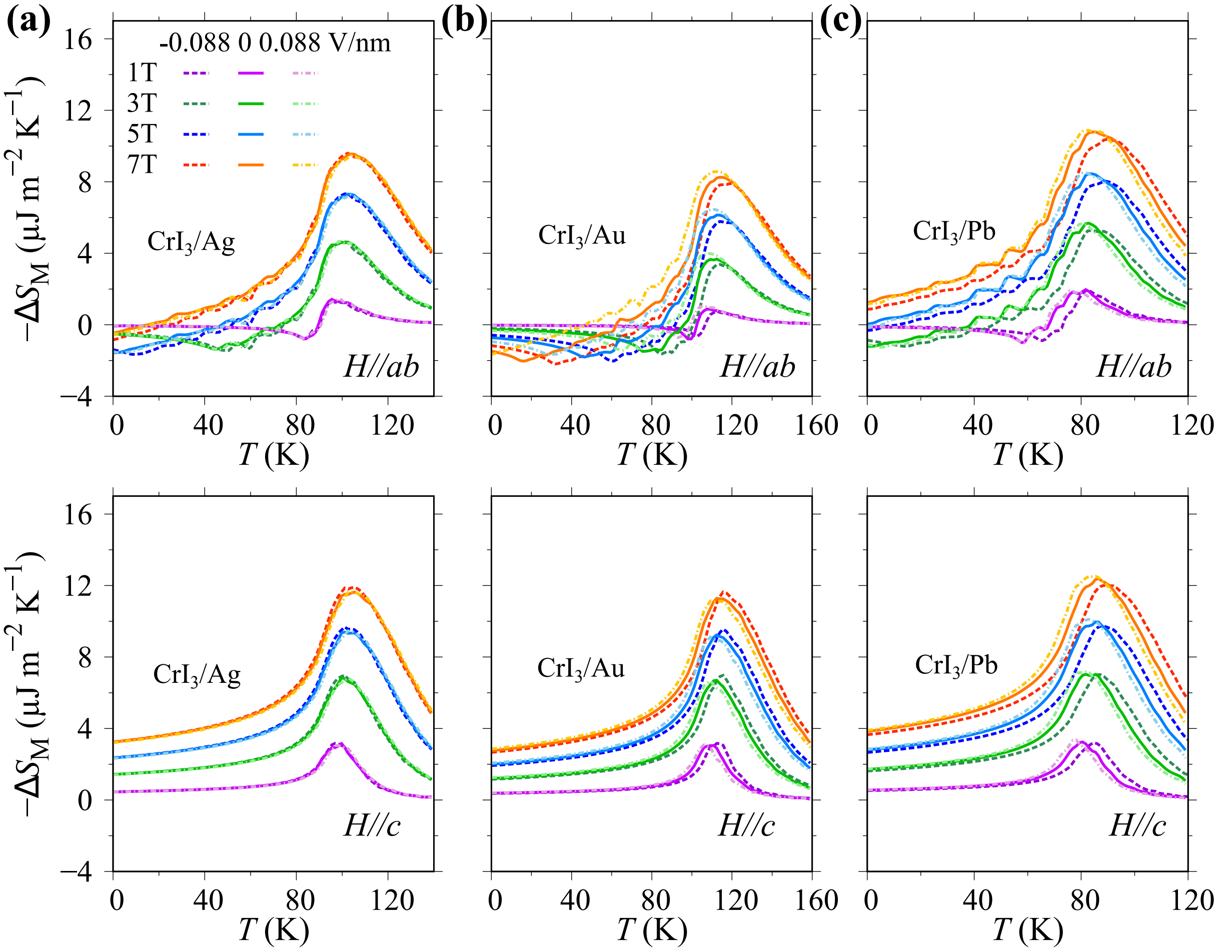


Fig. S6. Electric-field-tunable $-\Delta S_{\mathrm{M}}$ *vs* $T$ curves for (a) $CrI_3$/Ag heterostructure, (b) $CrI_3$/Au heterostructure, and (c) $CrI_3$/Pb heterostructure with magnetic field applied in different directions (top-row subfigures: $H//ab$, bottom-row subfigures: $H//c$).

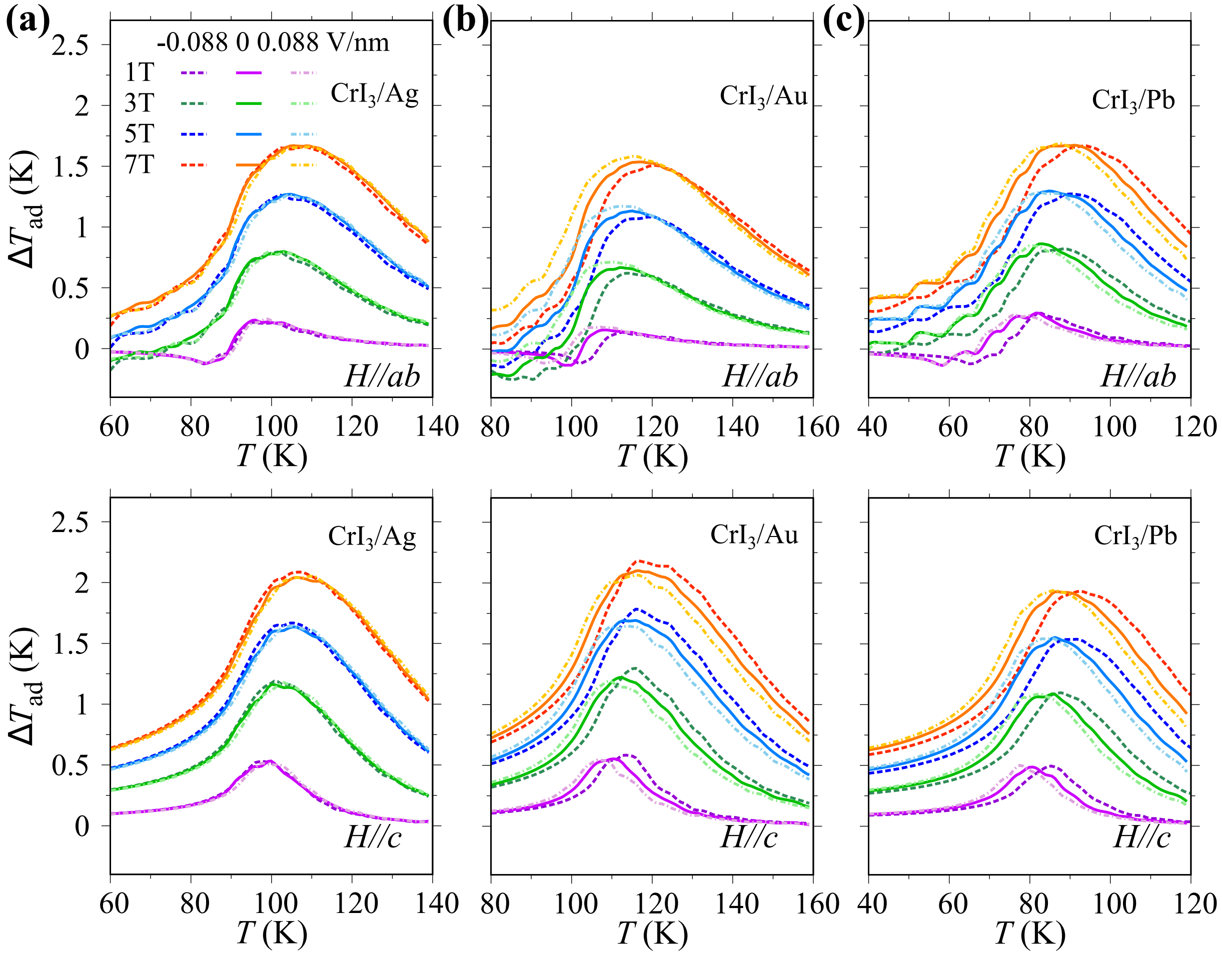


Fig. S7. Electric-field-tunable $\Delta T_{\mathrm{ad}}$ *vs* $T$ curves for (a) $\mathrm{CrI_3/Ag}$ heterostructure, (b) $\mathrm{CrI_3/Au}$ heterostructure, and (c) $\mathrm{CrI_3/Pb}$ heterostructure with magnetic field applied in different directions (top-row subfigures: $H//ab$, bottom-row subfigures: $H//c$).

## References

(1) Li, H.; Xu, Y. K.; Lai, K.; Zhang, W. B. The enhanced ferromagnetism of single-layer $CrX_3$ (X = Br and I) via van der Waals engineering. *Physical Chemistry Chemical Physics* **2019**, *21*, 11949–11955.
